# Supplementary material for: Women's Participation in Open Source Software: A Survey of the Literature
Source: arXiv:2105.08777 source file (2022-01-05)
Supplement: Supplementary file 1 [file appendixA.tex]

\appendix{Appendix A: Primary Studies without GL}\label{appendix-secondar-studies-without-gl}

%\noindent{\large\bfseries Included Secondary Studies References\par}
%\subsection{References}

\nocitesec{*}
%\bibliographystylesec{elsarticle-num}
\bibliographystylesec{appendixStyle}
\bibliographysec{secondaryStudiesNotIncluded}
